# Supplementary material for: Script-Strategy Aligned Generation: Aligning LLMs with Expert-Crafted Dialogue Scripts and Therapeutic Strategies for Psychotherapy
Source: arXiv:2411.06723 source file (2025-08-19)
Supplement: Supplementary file 1 [file appendix_consent.tex]

\clearpage

\begin{appendices}

\section{Consent for human evaluation study}
\label{appendix: consent}
\end{appendices}

\begin{table}[ht!]
\centering
\footnotesize

\begin{tabularx}{\textwidth}{>{\raggedright\arraybackslash}p{0.25\textwidth} >
{\raggedright\arraybackslash}X} 
\hline
\multicolumn{1}{l}{\textbf{\textcolor{black}{Human Evaluation}}} & \multicolumn{1}{l}{\textbf{}} \\
\hline
\textbf{Information Letter} & 
Dear participant, \newline \newline
Thank you for your interest in our study. This letter provides key information about the study's background and objectives.
\newline \newline
Study Background \newline
Our research evaluates the conversational agents (or chatbots) for psychotherapy. We aim to assess various AI agents based on real therapeutic dialogues, focusing on their application in health counseling, such as promoting healthy behaviors.
\newline \newline
Study Detail \newline
You are invited to participate in this study, lasting approximately 30 minutes, where you can freely interact with the conversational agents (or chatbots) within the health counseling scenarios. Your feedback is crucial for assessing the effectiveness of these AI agents. Please complete the survey in a quiet setting, focusing on the instructions and questions provided. There are no right or wrong answers; respond based on your personal perspective. If you encounter any issues or have questions, feel free to contact us.
\newline \newline 
Participation \newline
Your participation is voluntary. Surveys completed in under 15 minutes will be invalidated to ensure data quality. You will receive a \texteuro3 compensation upon completion.
\newline \newline
Discomfort, risks, and insurance \newline
We aim to minimize all potential risks during the study. You may withdraw from the study at any time without giving a reason. If you have any concerns, please communicate with the researcher.
\newline \newline
Your privacy is guaranteed \newline
Your privacy is our priority. No personal identifying information will be collected, and all data will remain confidential. Only the research team will access the data, and any published results will be anonymized.
\newline \newline
Further information \newline
Should you have questions about this study at any given moment, please contact the responsible researcher(s): [anonymous] \newline \newline
Thank you. 
\\ \hline

\textbf{Consent Form} &  
In this form, we reference the information letter detailing the research in which you are participating. By signing this form, you confirm that you understand the study's nature and methods as outlined in the information letter.
\newline \newline 
If you have any questions about this study, please contact the responsible researchers: [anonymous]. Formal complaints can be directed to the Ethics Review Board: [anonymous]. 
For questions or concerns about your personal data protection, please contact the Data Protection Officer: [anonymous].
\newline \newline 
By selecting ``Agree'' you confirm that:\newline 
• I am 18 years or older.\newline 
• I have read and understood the information letter.\newline 
• I agree to participate in the study and use the data obtained with it.\newline 
• I understand that I can withdraw the participation from the study at any moment without providing any reason. 
\\ \hline 
\end{tabularx}
\caption{The information letter and consent form used for human evaluation study according to ethical requirements of the institute.}
\end{table}
